# Supplementary material for: A Relational Intervention Approach for Unsupervised Dynamics Generalization in Model-Based Reinforcement Learning
Source: arXiv:2206.04551 source file (2022-06-09)
Supplement: Supplementary file 1 [file Appendix.pdf]

# Supplementary Material of “ A Relational Intervention Approach for Dynamics Generalization in Model-Based Reinforcement Learning ”

## A Appendix

We promise that we will public all codes after the acceptance of this paper.

### A.1 Environmental Settings

We follow the environmental settings of [3] in dynamics generalization. The details of settings are given as follows:

- **Pendulum** We modify the mass  $m$  and the length  $l$  of Pendulum to change its dynamics.  $\beta$  is 10.
- **Half-Cheetah** We modify the mass of regid link  $m$  and the damping of joint  $d$  of Half-Cheetah agent to change its dynamics.  $\beta$  is 1.
- **Crppled.Cheetah** We cripple the id of leg  $c$  of Half-Cheetah agent to change its dynamics.  $\beta$  is 1.
- **Ant** We modify the mass of ant’s leg  $m$  to change its dynamics. Specifically, we modify two legs by multiplying its original mass with  $m$ , and others two with  $\frac{1}{m}$ .  $\beta$  is 1.
- **Slim\_Humanoid** We modify the mass of rigid link  $m$  and the damping of joint  $d$  of the Slim\_Humanoid agent to change its dynamics.  $\beta$  is 1.
- **Hopper** We modify the mass of  $m$  of the Hopper agent to change its dynamics.  $\beta$  is 1.

The training and test modified parameter list can be found at the Table 1.

Table 1: The environmental settings in our paper.

|               | Training Parameter List                                                                                                                              | Test Parameter List                                                                                                      | Episode Length |
|---------------|------------------------------------------------------------------------------------------------------------------------------------------------------|--------------------------------------------------------------------------------------------------------------------------|----------------|
| Pendulum      | $m \in \{0.75, 0.8, 0.85, 0.90, 0.95, 1.1, 1.05, 1.1, 1.15, 1.2, 1.25\}$<br>$l \in \{0.75, 0.8, 0.85, 0.90, 0.95, 1.1, 1.05, 1.1, 1.15, 1.2, 1.25\}$ | $m \in \{0.2, 0.4, 0.5, 0.7, 1.3, 1.5, 1.6, 1.8\}$<br>$l \in \{0.2, 0.4, 0.5, 0.7, 1.3, 1.5, 1.6, 1.8\}$                 | 200            |
| Half-Cheetah  | $m \in \{0.75, 0.85, 1.00, 1.15, 1.25\}$<br>$d \in \{0.75, 0.85, 1.00, 1.15, 1.25\}$                                                                 | $m \in \{0.2, 0.3, 0.4, 0.5, 1.5, 1.6, 1.7, 1.8\}$<br>$d \in \{0.2, 0.3, 0.4, 0.5, 1.5, 1.6, 1.7, 1.8\}$                 | 1000           |
| C_Cheetah     | $c \in \{0, 1, 2, 3\}$                                                                                                                               | $c \in \{4, 5\}$                                                                                                         | 1000           |
| Ant           | $m \in \{0.85, 0.90, 0.95, 1.00\}$                                                                                                                   | $m \in \{0.20, 0.25, 0.30, 0.35, 0.40, 0.45, 0.50, 0.55, 0.60\}$                                                         | 1000           |
| Slim_Humanoid | $m \in \{0.80, 0.90, 1.00, 1.15, 1.25\}$<br>$d \in \{0.80, 0.90, 1.00, 1.15, 1.25\}$                                                                 | $m \in \{0.40, 0.50, 0.60, 0.70, 1.50, 1.60, 1.70, 1.80\}$<br>$d \in \{0.40, 0.50, 0.60, 0.70, 1.50, 1.60, 1.70, 1.80\}$ | 1000           |
| Hopper        | $m \in \{0.5, 0.75, 1.0, 1.25, 1.5\}$                                                                                                                | $m \in \{0.25, 0.375, 1.75, 2.0\}$                                                                                       | 500            |

## A.2 Training Details

Similar to the [3], we train our model-based RL agents and relational context encoder for 20 epochs, and we collect 10 trajectories by a MPC controller with 30 horizon from environments at each epoch. In addition, the cross entropy method (CEM) with 200 candidate actions is chosen as the planning method. Specifically, the batch size for each experiment is 256. All module are learned by a Adam optimizer with 0.001 learning rate.

## A.3 Network Details

Similar to the [3], the relational encoder is constructed by a simple 3 hidden-layer MLP, and the output dim of environmental-specific vector  $\hat{z}$  is 10. The relational head is modelled as a single layer MLP with 10 units (same with the dim of  $\hat{z}$ ) and an output layer. The dynamics prediction model is a 4 hidden-layer MLP with 200 units.

## A.4 Visualization

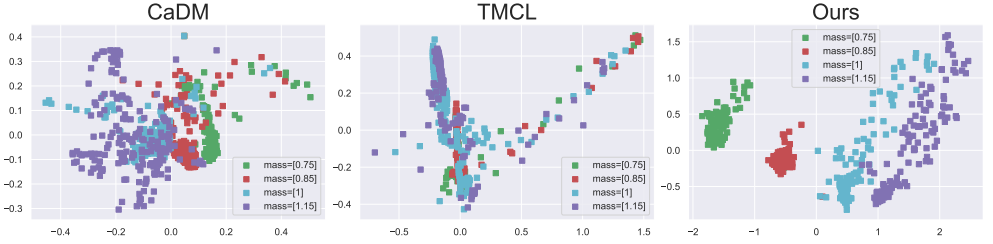

Figure 1: The PCA of estimated context (environmental-specific) vectors in **Pendulum** task.

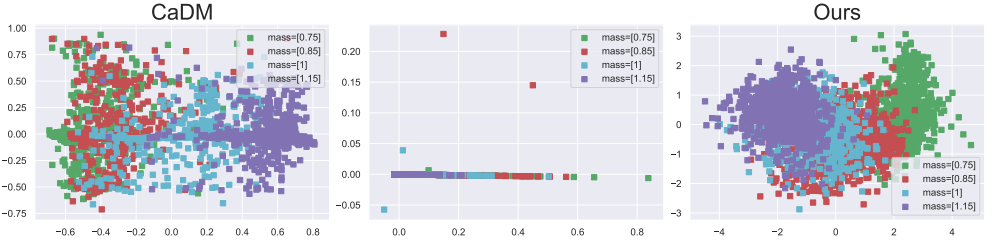

Figure 2: The PCA of estimated context (environmental-specific) vectors in **HalfCheetah** task.

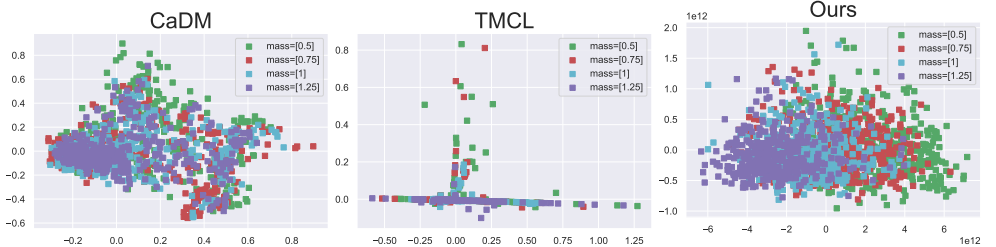

Figure 3: The PCA of estimated context (environmental-specific) vectors in **Hopper** task.

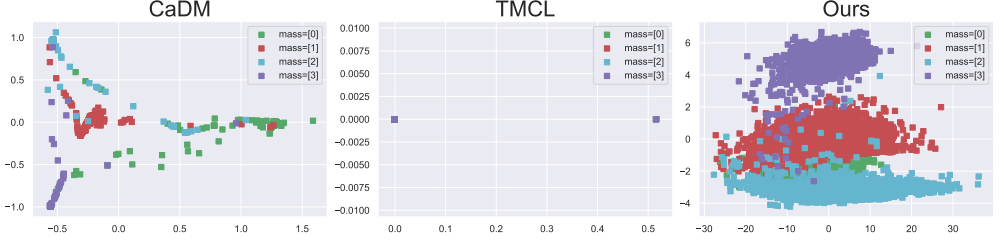

Figure 4: The PCA of estimated context (environmental-specific) vectors in **Cripple\_Halfcheetah** task.

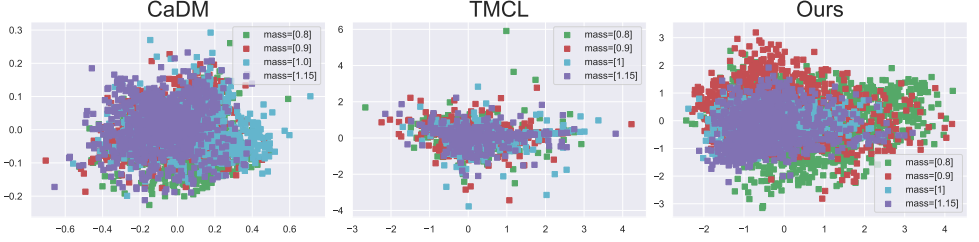

Figure 5: The PCA of estimated context (environmental-specific) vectors in **Slim\_Humanoid** task.

## References

- [1] Chelsea Finn, Pieter Abbeel, and Sergey Levine. Model-agnostic meta-learning for fast adaptation of deep networks. In *International Conference on Machine Learning*, pages 1126–1135. PMLR, 2017.
- [2] Thanard Kurutach, Ignasi Clavera, Yan Duan, Aviv Tamar, and Pieter Abbeel. Model-ensemble trust-region policy optimization. *arXiv preprint arXiv:1802.10592*, 2018.
- [3] Kimin Lee, Younggyo Seo, Seunghyun Lee, Honglak Lee, and Jinwoo Shin. Context-aware dynamics model for generalization in model-based reinforcement learning. In *International Conference on Machine Learning*, pages 5757–5766. PMLR, 2020.
- [4] Anusha Nagabandi, Ignasi Clavera, Simin Liu, Ronald S Fearing, Pieter Abbeel, Sergey Levine, and Chelsea Finn. Learning to adapt in dynamic, real-world environments through meta-reinforcement learning. *arXiv preprint arXiv:1803.11347*, 2018.
- [5] Anusha Nagabandi, Chelsea Finn, and Sergey Levine. Deep online learning via meta-learning: Continual adaptation for model-based rl. *arXiv preprint arXiv:1812.07671*, 2018.
- [6] Younggyo Seo, Kimin Lee, Ignasi Clavera, Thanard Kurutach, Jinwoo Shin, and Pieter Abbeel. Trajectory-wise multiple choice learning for dynamics generalization in reinforcement learning. *arXiv preprint arXiv:2010.13303*, 2020.
